# Supplementary material for: Magnetic and Structural Properties of 5d Osmate Double Perovskites Probed by Nuclear Magnetic Resonance
Source: arXiv:2303.07573 source file (2023-03-14)
Supplement: Supplementary file 1 [file appendix.tex]

%\begin{appendices}

%Some Table of Contents entry formatting
%\addtocontents{toc}{\protect\renewcommand{\protect\cftchappresnum}{\appendixname\space}}
%\addtocontents{toc}{\protect\renewcommand{\protect\cftchapnumwidth}{6em}}

%Begin individual appendices, separated as chapters

%\end{appendices}
\newpage
\section*{References}
{
%\bibliographystyle{unsrt}
%\bibliography{journals,phd-references}
\bibliographystyle{apsrev4-1}
%\printbibliography
\bibliography{bib}
}
